# Supplementary material for: Three counterexamples to a conjecture of Colin de Verdi\`ere on multiplicity
Source: arXiv:2312.03504 ancillary file (2026-06-16)
Supplement: Supplementary file 1 [file generate_classes.pdf]

## generate\_classes

December 5, 2023

```
[1]: # This file computes conjugacy classes of primitive hyperbolic elements up to a
      ↪given translation length
      # in a given (2,3,r)-triangle group

      # Counterclockwise rotation of angle theta around the point i
      def rot(theta):
          return matrix(RBF, [[cos(-theta/2), -sin(-theta/2)], [sin(-theta/2), cos(-theta/
          ↪2)]]))

      # Upward hyperbolic translation of length t along imaginary axis
      def up(t):
          return matrix(RBF, [[exp(t/2), 0], [0, exp(-t/2)]])

      # Act on the point w by the matrix mat as a Mobius transformation
      def apply_mobius(mat, w):
          a=mat[0][0]
          b=mat[0][1]
          c=mat[1][0]
          d=mat[1][1]
          return (a*w+b)/(c*w+d)

      # A class for elements of a (p,q,r)-triangle group. We represent elements as
      # 1) sequences of integers that encode the element as a product in the
      ↪generators,
      # where 1 represents x, 2 represents y, 3 represents z, inverses are indicated
      ↪by negatives
      # 2) 2 by 2 matrices with entries in RBF
      # In addition, each element can be given a state for use in the automaton

      class element:

          # Initiate an instance of the class element. All the attributes are
          ↪optional.
          def __init__(self, sequence=None, mat=None, state=None):
              self.as_sequence = sequence
              self.as_matrix = mat
              self.state = state
```

```

# Multiply two elements
def __mul__(self, other):
    prod = element()
    prod.as_sequence = self.as_sequence+other.as_sequence # This is
    ↪ concatenation of the sequences
    prod.as_matrix = self.as_matrix*other.as_matrix

    return prod

# Raise element self to the power other
def __pow__(self, other):
    if other==1:
        return self
    elif other>1:
        return self*self^(other-1)

    # We do not use negative powers in the program

# Act by the element as a Mobius transformation on the point w
def as_mobius(self, w):
    return apply_mobius(self.as_matrix, w)

# Return the absolute trace of the element self
def trace(self):
    return abs(self.as_matrix.trace())

# Return true if the upper bound on the absolute trace of the element is
    ↪ larger than 2, False otherwise.
def might_be_hyperbolic(self):
    if not self.trace()<=2:
        return True
    else:
        return False

# Return true if the lower bound on the absolute trace of the element is
    ↪ larger than 2, False otherwise.
def is_hyperbolic(self):
    if self.trace()>2:
        return True
    else:
        return False

# Return the translation length of self
def length(self):
    T = self.trace()

```

```

    if T>2:
        return 2*arccosh(T/2)
    elif T<=2:
        return 0
    else:
        # In this case the ball T overlaps 2 so the element could be
        ↪hyperbolic a priori.
        # We replace T's lower bound by 2 in that case.
        return RBF(2*arccosh(RIF(2,T.upper())/2))

# Given 2 points z and w in the upper half-plane, this computes cosh of the
↪distance between them.
def pre_dist(z,w):
    return RBF(1+abs(z-w)^2/(2*imag(z)*imag(w)))

# Compute the hyperbolic distance between z and w in the upper half-plane.
def dist(z,w):
    P = pre_dist(z,w)
    if not P>=1:
        # This cannot happen in principle, but it sometimes does due to
        ↪rounding.
        # In that case, we replace the lower bound in P by 1.
        P = RIF(1,P.upper())
    return RBF(arccosh(P))

# Compute the distance from a point to the translation axis of f, where f is an
↪instance of the class element.
def dist_to_axis(point,f):
    if not f.is_hyperbolic():
        print('Error, element not hyperbolic.')
        return

    L = f.length()
    M = dist(point,f.as_mobius(point))

    c = sinh(M/2)/sinh(L/2)

    if c>=1:
        return arccosh(sinh(M/2)/sinh(L/2))
    else:
        # This means that point is nearly on the axis. We replace the lower bound
        ↪on distance by zero.
        return RBF(arccosh(RIF(1,c.upper())))

# Compute (a lower bound on) the distance between a point x and a geodesic
↪segment seg (given by the list of its endpoints)

```

```

def dist_point_segment(x,seg):

    # We form a triangle with x and the segment, compute its side lengths and
    ↪interior angles
    y = seg[0]
    z = seg[1]
    a = dist(y,z)
    b = dist(x,z)
    c = dist(x,y)
    gamma = arccos((cosh(a)*cosh(b)-cosh(c))/(sinh(a)*sinh(b))) # angle at z
    beta = arccos((cosh(a)*cosh(c)-cosh(b))/(sinh(a)*sinh(c))) # angle at y
    alpha = arccos((cosh(c)*cosh(b)-cosh(a))/(sinh(c)*sinh(b))) # angle at x

    # If one of the angles at y or z is obtuse, then the orthogonal projection
    ↪of x onto the geodesic through y and z
    # falls outside the segment, and the minimal distance is achieved at an
    ↪endpoint of the segment
    if beta > RBF(pi/2):
        return c
    elif gamma > RBF(pi/2):
        return b

    # Otherwise, the minimal distance is given by the orthogonal projection and
    ↪we use Formula 2.2.2(iii) in Buser's book.
    # Note that it is possible for both inequalities above to evaluate to
    ↪false, but for one angle to still be larger than pi/2 (because beta and
    ↪gamma are intervals).
    # In these cases, the formula below still gives a lower bound on the
    ↪distance (it is the distance to the complete geodesic through seg)
    else:
        return arcsinh(sin(gamma)*sinh(b))

# Determine if two elements f and g of a triangle group are equal by computing
    ↪their values on a pair of triangle vertices
# min_dist is the smallest distance between two distinct triangle vertices in
    ↪the tiling.
def are_equal(f,g,vertex1,vertex2,min_dist):
    p1=pre_dist(f.as_mobius(vertex1),g.as_mobius(vertex1))
    p2=pre_dist(f.as_mobius(vertex2),g.as_mobius(vertex2))

    if p1<cosh(min_dist) and p2<cosh(min_dist): #This means both pairs of
    ↪images agree for sure.
        return True
    elif p1>1 or p2>1: #This means at least one pair disagrees for sure.
        return False
    else: #This means there is too much imprecision on the images to be certain.
        print('Error: Not enough precision to solve the word problem.')

```

```

    return

# Test if two elements f and g are conjugate via an element in the list
↳ conjugators.
# We still use two distinct vertices in the tiling and half the smallest
↳ possible pairwise distance to test.
def are_conjugate(f,g,conjugators,vertex1,vertex2,min_dist):
    for h in conjugators:
        if are_equal(h*f,g*h,vertex1,vertex2,min_dist):
            return True
    return False

# Combine the lists in a list of list into a single list.
def combine_lists(W):
    L = []
    for lst in W:
        L+=lst
    return L

# Given a list L of elements of a (p,q,r)-triangle group, only keep the
↳ elements that are hyperbolic,
# whose translation length is at most lmax, and whose translation axis passes
↳ within distance D of the point i
def keep_hyper(L,lmax,D,p,q,r,vertex1,vertex2,min_dist):

    newL = []
    m = lcm([p,q,r])
    identity = element([],matrix([[1,0],[0,1]]))

    for elem in L:
        if elem.might_be_hyperbolic() and not elem.length()>lmax:
            if elem.is_hyperbolic():
                if not dist_to_axis(i,elem)>D:
                    newL.append(elem)

            else:
                # This means elem is probably elliptic (we only work with
↳ cocompact triangle groups so there are no parabolics)
                # We test for ellipticity.

                if not are_equal(elem^m,identity,vertex1,vertex2,min_dist):
                    print("Error: There is a hyperbolic element whose axis we
↳ cannot compute.")
                    return

    return newL

```

```

# Group hyperbolic elements from a list according to their translation length,
↳ up to a certain tolerance.
# Return a dictionary whoses keys are approximate translation lengths and whose
↳ entries are the corresponding groups of elements.
def regroup(W,tol=0.001):
    dict = {}
    for elem in W:
        if elem.length().rad()>tol:
            print("Error: The lengths are not precise enough for the given
↳ tolerance.")
            return

        found = False
        for key in dict.keys():
            # If the length is already there up to the tolerance, add elem to
↳ the list of elements with that approximate trace.
            if key-tol<=elem.length().center()<=key+tol:
                dict[key].append(elem)
                found = True
                break
            # Otherwise, create a new list.
        if found==False:
            dict[elem.length().center()]=[elem]

    return dict

# Given a dictionary H of hyperbolic elements grouped by length, filter each
↳ group to keep one representative of each conjugacy class.
# conjugators is a list of elements sufficient to test for conjugacy.
def classes(H,conjugators,vertex1,vertex2,min_dist):

    keys=H.keys()

    for key in keys:
        length = len(H[key])
        j = 0
        while j < length: #for each element in the list H[key], suppress its
↳ conjugates that come afterwards
            f = H[key][j]

            k = j+1
            while k < length:
                g = H[key][k]
                if are_conjugate(f,g,conjugators,vertex1,vertex2,min_dist):
                    H[key].pop(k)

```

```

        length = length-1
    else:
        k = k+1
    j = j+1

    return H

# Delete non-primitive elements in the dictionary H which is assumed to contain
↳ only one representative of each conjugacy class.
# We test if elements are conjugate to powers using the list of conjugators.
def delete_powers(H, conjugators, vertex1, vertex2, min_dist):

    keys = H.keys()

    if len(keys)==0:
        return H
    else:
        # We make a list of true lower and upper bounds on translation lengths
↳ for elements in H
        lower_keys = []
        upper_keys = []

        for key in keys:
            upper_bound = 0
            lower_bound = Infinity
            for elem in H[key]:
                if elem.length().upper()>upper_bound:
                    upper_bound = elem.length().upper()
                if elem.length().lower()<lower_bound:
                    lower_bound = elem.length().lower()

            upper_keys.append(upper_bound)
            lower_keys.append(lower_bound)

        max_length = max(upper_keys)

    n = 0
    for key in keys:
        lower_key = lower_keys[n]
        upper_key = upper_keys[n]
        k = 2
        while k*lower_key < max_length: # We go through multiples of lengths
↳ as long as it doesnt surpass the maximum in the list
            N=0
            for mult in keys: # For each length in the list we check if it can
↳ be a k times the length of an element in H[key]

```

```

        # We check if the elements in H[mult] are potentially k powers
        ↪ of elements in H[key]
        if not k*RBF(RIF(lower_key,upper_key))!=
        ↪ RBF(RIF(lower_keys[N],upper_keys[N])):
            # This means the intervals overlap so mult is potentially a
            ↪ multiple of key, so we check all pairs to delete the powers
            for elem1 in H[key]:

                length = len(H[mult])
                j = 0
                while j < length:
                    elem2 = H[mult][j]
                    if
        ↪ are_conjugate(elem1^k,elem2,conjugators,vertex1,vertex2,min_dist):
                        H[mult].pop(j)
                        length = length-1
                        break # At most one element can be the k-th
        ↪ power of H by hypothesis, so we break after finding one
                    else:
                        j = j+1

            N = N+1

        k = k+1
        n = n+1
    return H

# Compute the total number of elements in a disctionary of lists.
def number_elem(W):
    N = 0
    for key in W.keys():
        N+=len(W[key])

    return N

# Convert a dictionary to a list
def dict_to_list(W):
    L=[]
    for M in W.values():
        L+=M

    return L

# Return only the sequences of the elements in a list
def sequences(W):
    return [elem.as_sequence for elem in W]

```



```

# Generate conjugacy classes of primitive hyperbolic elements in the
↳ (2,3,r)-triangle group up to translation length lmax.
# The function returns one representative of each conjugacy class, given as a
↳ sequence (list) of  $\pm 1$  (for  $x^{\pm 1}$ ),  $\pm 2$  (for  $y^{\pm 1}$ ),  $\pm 3$  (for  $z^{\pm 1}$ ).
def generate(r,lmax):
    lmax = RBF(lmax)

    p=2
    q=3

    # interior angles of the triangle
    alpha = pi/p
    beta = pi/q
    gamma = pi/r

    # side lengths
    a = RBF(arccosh((cos(alpha)+cos(beta)*cos(gamma))/(sin(beta)*sin(gamma))))
    b = RBF(arccosh((cos(beta)+cos(alpha)*cos(gamma))/(sin(alpha)*sin(gamma))))
    c = RBF(arccosh((cos(gamma)+cos(alpha)*cos(beta))/(sin(alpha)*sin(beta))))

    # We position our base triangle with vertex C at i, than A above C on the
↳ imaginary axis, and B in the second quadrant.

    # triangle vertices
    C = i
    A = apply_mobius(up(b),i)
    B = apply_mobius(rot(gamma)*up(a),i)

    # rotation matrices by twice the interior angles (X is the rotation at A, Y
↳ the rotation at B and Z the rotation at C)
    X = up(b)*rot(2*alpha)*up(-b)
    Y = rot(gamma)*up(a)*rot(2*beta)*up(-a)*rot(-gamma)
    Z = rot(2*gamma)

    # minimum distance between triangle vertices
    min_dist = min([a,b,c])

    # Since p=2, the diameter of the triangle is the hypotenuse a opposite to
↳ the vertex A.
    # The same is true for the fundamental domain Dom obtained by pairing the
↳ base triangle with its reflection in the imaginary axis.
    # We add a small amount to the diameter to deal with potential translation
↳ axes that are nearly tangent to the disk of radius a.
    D = a+RBF(0.001)

```

```

# element_target is how far we need to go to generate all hyperbolic
↳elements with translation length at most lmax,
# in term of how much i is displaced
element_target = 2*arcsinh(cosh(D)*sinh(lmax/2))

# conjugacy_target is how far we need to look for a conjugating element, in
↳terms of how much i is displaced
conjugacy_target = 2*arccosh(cosh(D)*cosh(lmax/4))

# This is a the side of the fundamental domain Dom opposite to the vertex C
↳at i.
# We use images of this segment to compute the inner radius of the region
↳covered so far
segment =
↳[apply_mobius(rot(-gamma)*up(a),i),apply_mobius(rot(gamma)*up(a),i)]

# layers is a list of lists of elements in the triangle group.
# Each sublists represents a layer of regular r-gons in the tiling.
# We start with the central r-gon, then each layer is generated using the
↳previous one.
layers = [[element([3]*j,Z^j,'M') for j in range(r)]]

# length_covered is the inner radius of the region covered so far, measured
↳from the point i.
length_covered = b

# We first generate enough elements to cover element_target
while not length_covered >= element_target or not length_covered >=
↳conjugacy_target :
    children = []
    for parent in layers[-1]:

        if parent.state=='M': #these have r-4 active children

            for j in range(r):
                child = element(parent.as_sequence+[1]+[3]*j,parent.
↳as_matrix*X*Z^j)
                if j==2:
                    child.state = 'R'
                elif 3<=j<r-2:
                    child.state = 'M'
                elif j==r-2:
                    child.state = 'L'
                else:
                    child.state = 'I'
                children.append(child)

```

```

elif parent.state=='L': #these have r-5 active children

    for j in range(r):
        child = element(parent.as_sequence+[1]+[3]*j,parent.
↪as_matrix*X*Z^j)
        if j==2:
            child.state = 'R'
        elif 3<=j<r-3:
            child.state = 'M'
        elif j==r-3:
            child.state = 'L'
        else:
            child.state = 'I'
        children.append(child)

layers.append(children)

# We compute (a lower bound on) the inner radius of the region covered
↪so far by finding the minimum distance to a boundary segment.
# The segments on the boundary are those on the last layer whose state
↪is not 'I'.
length_covered = Infinity
for elem in layers[-1]:
    if elem.state!='I':
        s = dist_point_segment(i,[elem.as_mobius(u) for u in segment])
        if not s > length_covered:
            length_covered = RBF(s.lower())

# Combine the layers in a single list
conjugators = combine_lists(layers)

# Only keep hyperbolic elements of translation length at most lmax whose
↪axis intersects the disk of radius D around i
elements = keep_hyper(conjugators,lmax,D,p,q,r,C,A,min_dist) #This
↪function creates a copy of the list so it does not modify the conjugators

# Regroup them according to translation length
elements = regroup(elements)

# Keep only one representative of each conjugacy class
cl = classes(elements,conjugators,C,A,min_dist)

# Delete powers
prim = delete_powers(cl,conjugators,C,A,min_dist)

# Convert to list

```

```

prim = dict_to_list(prim)

# Check that the inequalities required to solve the conjugacy problem were
→indeed verified for all elements.
# In the keep_hyper function above we only checked that the reverse
→inequalities were not False to detect all elements for sure.
for elem in prim:
    if not dist_to_axis(i,elem)<=D:
        print('One translation axis is almost tangent to the boundary of'
        →the disk of radius D.')
        print(D,dist_to_axis(i,elem))
        return

    elif not elem.length()<=lmax:
        print('The cutoff lmax is too close to a translation length. Change'
        →it slightly.')
        return

return sequences(prim)

```

```

[2]: P = generate(8,3.0)
      print(P)

```

```

[[1, 3, 3, 3], [1, 3, 3, 3, 3], [1, 3, 3, 3, 1, 3, 3, 3], [1, 3, 3, 3, 3, 1,
3, 3, 3, 3, 3], [1, 3, 3, 3, 1, 3, 3, 3, 3, 3], [1, 3, 3, 3, 1, 3, 3, 3, 3, 3,
3], [1, 3, 3, 3, 3, 3, 3, 1, 3, 3]]

```

```

[3]: P = generate(7,3.0)
      print(P)

```

```

[[1, 3, 3, 3], [1, 3, 3, 3, 1, 3, 3, 3, 3], [1, 3, 3, 3, 3, 3, 1, 3, 3], [1, 3,
3, 3, 1, 3, 3, 3, 1, 3, 3, 3, 3, 3], [1, 3, 3, 3, 1, 3, 3, 3, 3, 3, 1, 3, 3],
[1, 3, 3, 3, 1, 3, 3, 3, 3, 3, 3, 1, 3, 3, 3, 3]]

```

```

[ ]:

```
