# Supplementary material for: Three counterexamples to a conjecture of Colin de Verdi\`ere on multiplicity
Source: arXiv:2312.03504 ancillary file (2026-06-16)
Supplement: Supplementary file 3 [file verify_genus_17.pdf]

# verify\_genus\_17

December 5, 2023

[1]:

```
#####
# -----
# Constants
# -----
#####

# The parameters that determine a triangle group
p=2
q=3
r=7

#####
# -----
# Group theory input
# -----
#####

# The Deck group of the surface
# - A free group of rank 3:
F = FreeGroup(3)
F.inject_variables()

# - Deck group
# Its presentation was found by M. Conder and is available at:
# https://www.math.auckland.ac.nz/~conder/TriangleGroupQuotients101.txt
# The group appears as T17.1 in Conder's list
G = F / (x0^2, x1^3, x0 * x1 * x2, x2^-3 * x0 * x1 * x2^-3, x0 * x2 * x1 * x0 *
↪ x2 * x1 * x0 * x1^-1 * x2^-1 * x0 * x1^-1 * x2^-1 * x0 * x1^-1 * x2^-1 * x0
↪ x1^-1 * x2^-1 * x0 * x1^-1 * x2^-1 * x0 * x1^-1 * x2^-1, x2 * x1 * x0 * x2
↪ x1 * x2^-1 * x0 * x2 * x1^-1 * x2^-1 * x0 * x1^-1 * x2^-2 * x0 * x2 *
↪ x1^-1 * x2^-1 * x0 * x1^-1 * x2^-2 * x0 * x2)

# - The list of characters of G:
characters = G.gap().Irr()

# - Printing the orders of the generators in the group G. If these are p, q and
↪ r respectively,
```

```

# then this implies the corresponding subgroup of  $T(p,q,r)$  has no torsion
print("\nOrders of the generators of G:")
print(G(x0).order())
print(G(x1).order())
print(G(x2).order())

# - Printing the genus
genus = 1 + (1-1/p-1/q-1/r)*G.order()/2
print("\nThe genus of the corresponding surface is", genus)

print("\nGAP recognizes the group G as",G.gap().StructureDescription())

```

Defining x0, x1, x2

Orders of the generators of G:

2  
3  
7

The genus of the corresponding surface is 17

GAP recognizes the group G as  $(C2 \times C2 \times C2) \cdot \text{PSL}(3,2)$

```

[2]: # - Determine which complex representations associated to the characters
# can be realized as a real representation and which can't.
# This computation is based on Proposition 39 (p. 109) in:
# "Linear Representations of Finite Groups" by J.-P. Serre (1977)
# This computation is in a separate cell because it takes a lot of time.
is_real = []
for m in range(len(characters)):
    phi = characters[m]
    S = 0
    for g in G.gap().List():
        S += (g^2)^phi

    # If  $S > 0$ , then the complex representation can be realized as a real
    ↪representation
    # whose character equals the complex character
    if S > 0:
        is_real += [True]
    # If not, the complex representation gives rise to an irreducible real
    ↪representation
    # whose character equals twice the real part of the complex character
    else :
        is_real += [False]
is_real

```

```
[2]: [True, False, False, True, True, True, True, True, True, True, True]
```

```
[2]: # Because of the time it takes to compute it, we feed the output from the
      ↪ previous cell into this cell
is_real = [True, False, False, True, True, True, True, True, True, True, True]

# A function that computes the real character of a group element
# Input:
# * g: an element of G, represented as a list
# * m: an natural number between 0 and len(characters)-1
def Character(g,m):
    phi = characters[m]
    elt = G(1)
    for t in range(len(g)):
        if g[t] == 1:
            elt = elt * G(x0)
        elif g[t] == 2:
            elt = elt * G(x1)
        elif g[t] == 3:
            elt = elt * G(x2)
        elif g[t] == -1:
            elt = elt * G(x0)^(-1)
        elif g[t] == -2:
            elt = elt * G(x1)^(-1)
        elif g[t] == -3:
            elt = elt * G(x2)^(-1)
    if is_real[m] == True:
        # return the character as a real number as opposed to something that
        ↪ lives in GAP
        return RBF((elt.gap())^phi)
    else:
        return CBF((2*(elt.gap())^phi).sage()).real()

# Functions to compute the Fuchsian matrix representation
# - The counter clockwise rotation of the hyperbolic plane fixing i and of
      ↪ angle theta
def rot(theta):
    return matrix(RBF,[[cos(-theta/2),-sin(-theta/2)],[sin(-theta/2),cos(-theta/
      ↪ 2)]]))

# - Moving up by distance t along the imaginary axis
def up(t):
    return matrix(RBF,[[exp(t/2),0],[0,exp(-t/2)]]))

# - Angles
alpha = pi/p
beta = pi/q
```

```

gamma = pi/r

# - Lengths
a = RBF(arccosh((cos(alpha)+cos(beta)*cos(gamma))/(sin(beta)*sin(gamma))))
b = RBF(arccosh((cos(beta)+cos(alpha)*cos(gamma))/(sin(alpha)*sin(gamma))))
c = RBF(arccosh((cos(gamma)+cos(alpha)*cos(beta))/(sin(alpha)*sin(beta))))

# - The images of the generators of the triangle group as rotation matrices
X = up(b)*rot(2*alpha)*up(-b)
Y = rot(gamma)*up(a)*rot(2*beta)*up(-a)*rot(-gamma)
Z = rot(2*gamma)

# A function that computes the Fuchsian representation, as matrices with
  ↪ coefficients in FIELD
#   Input:
#   * g: an element of the triangle group, represented as a list
def Fuchsian(g):
    M = matrix(RBF,[[1,0],[0,1]])
    for t in range(len(g)):
        if g[t] == 1:
            M = M * X
        elif g[t] == 2:
            M = M * Y
        elif g[t] == 3:
            M = M * Z
        elif g[t] == -1:
            M = M * X^(-1)
        elif g[t] == -2:
            M = M * Y^(-1)
        elif g[t] == -3:
            M = M * Z^(-1)
    return M

# A function that computes the trace of an element
#   Input:
#   * g: an element of the triangle group, represented as a list
def Trace(g):
    M = Fuchsian(g)
    return M.trace()

```

[3]:

```

#####
# -----
#   Test function
# -----
#####

```

```

# - The fourth convolution power of the normalized characteristic function of  $\chi_{[-d,d]}$ 
# i.e.  $f$ 
def f(d,y) :
    if (y >= 0) :
        y = -y
    if (y <= -4*d) :
        return 0
    elif ((y >= -4*d) and (y <= -2*d)) :
        return (1/(12*d)) * (2 + y/(2*d))^3
    elif ((y >= -2*d) and (y <= 0)) :
        return (4 - 6*(y/(2*d))^2 - 3*(y/(2*d))^3)/(12*d)

```

[4] : #####

```

# -----
# Contributions to the Selberg trace formula
# -----
#####

# Error term in the degree  $2N-2$  Taylor approximation of  $x/\sinh(x/2)$ 
def taylor_err(x,N):
    return 8*(x/2*pi)^N / (1-1/(2*pi)^2)

# A function to compute the integral contribution in the STF
# Input:
# * d: the half width of the support of  $h$ 
# * m: the index of the character
def integral_contribution(d,m):
    # Size of an interval on which we use the taylor approximation of  $1/\sinh$  in
    # one of the integrals below
    width = 1/(10^10)

    D = QQ(d)

    # Integrate  $f'(x)/\sinh(x/2)$ 
    #  $f'$  has two different definitions on two intervals
    # On top of that, near 0, we need to deal with the division by  $\sinh(x/2)$ 

    #Zeroth term: the integral on a small interval near 0

    # -Estimate for the integral of the error in the Taylor approximation of
    #  $f'(x)/\sinh(x/2)$  on the interval  $[0,width]$ 
    ErrorTerm = width*taylor_err(width,4) * (1/(4*D^3) + 3*width/(32*D^4))
    I = RBF(RIF(-ErrorTerm,ErrorTerm))

```

```

    # Integrate Taylor approximation of  $f'(x)/\sinh(x/2)$  over the interval  $[0, width]$ 
    I += -CBF.integral(lambda x, _: (2-x^2/12+7*x^4/2880-31*x^6/483840)*(-x)/(32*D^4), 0, width)

    # First term: the integral on the first domain of definition of  $f'$ 
    I += -CBF.integral(lambda x, _: (-x/(4*D^3) + 3*x^2/(32*D^4))*(1/sinh(x/2)), width, 2*D)

    # Second term: the integral on the second domain of definition of  $f'$ 
    I += -CBF.integral(lambda x, _: -(2-x/(2*D))^2/(8*D^2*sinh(x/2)), 2*D, 4*D)

    # Character([], m) is the complex dimension of the irrep
    cst = Character([], m)*(1-1/p-1/q-1/r)
    return cst * I

# A function to compute the elliptic contribution in the STF
# Input:
# * d: the half width of the support of the characteristic function that we use to define f
# * m: the index of the character
def elliptic_contribution(d, m):
    orders = [p, q, r]
    contrib = 0
    D = QQ(d)
    for o in range(3):
        for t in range(1, orders[o]):
            theta = RBF(pi*t/orders[o])

            # Computing the integral:

            # First term: the integral on the first domain of definition of f
            def h(x):
                return (4-6*(x/(2*D))^2+3*(x/(2*D))^3)/(12*D)
            I = CBF.integral(lambda x, _: h(x)*cosh(x/2)/(cosh(x)-1+2*sin(theta)^2), 0, 2*D)

            # Second term: the integral on the second domain of definition of f
            def h(x):
                return (2-x/(2*D))^3/(12*D)
            I += CBF.integral(lambda x, _: h(x)*cosh(x/2)/(cosh(x)-1+2*sin(theta)^2), 2*D, 4*D)

            cst = Character(t*[o+1], m) / orders[o]

            contrib += cst * I

```

```

    return contrib

# A function to compute the hyperbolic contribution in the STF
# Input:
# * d: the half width of the support of the characteristic function that we use
    ↳ to define f
# * m: the index of the character
# * prim_hyp_elts: a list of primitive hyperbolic elements
# * L: an upper bound for the translation lengths that are included
#     NB: for the program to produce sensible output, it is necessary that
    ↳ prim_hyp_elts contains
#         all primitive hyperbolics in the group of translation length at most
    ↳ L
#         and that the support of the  $f^{\wedge}$  defined above is contained in  $[-L, L]$ .
#         This is not checked in this function.
def hyperbolic_contribution(d,m,prim_hyp_elts,L):

    contrib = 0
    D = QQ(d)

    for g in prim_hyp_elts:

        length = 2*acosh(abs(Trace(g))/2)
        t = 1

        while t*length.upper() <= L:
            char = Character(t*g,m)

            contrib += char*length*f(D,t*length)/(2*sinh(t*length/2))

            t += 1
    return contrib

```

[7]:

```

#####
# -----
#   V e r i f i c a t i o n
# -----
#####

# A rational polynomial ring in which we will perform Sturm's method
P.<x> = PolynomialRing(QQ)
K = 100 # a cut off for the degree of a Taylor approximation we will apply

# The output of generate_classes:
# The list of conjugacy classes in the (p,q,r) (orientable) triangle group whose
# translation length is at most L, all represented by one of their elements.

```

```

prim_hyp_elts = [[1, 3, 3, 3],
                 [1, 3, 3, 3, 1, 3, 3, 3, 3],
                 [1, 3, 3, 3, 3, 3, 1, 3, 3],
                 [1, 3, 3, 3, 1, 3, 3, 3, 1, 3, 3, 3, 3],
                 [1, 3, 3, 3, 1, 3, 3, 3, 3, 3, 1, 3, 3],
                 [1, 3, 3, 3, 1, 3, 3, 3, 3, 3, 1, 3, 3, 3, 3]]

L = 3

# The bound on the maximal possible spectral gap of a closed hyperbolic surface
# of genus 17, that
# we proved in "Linear programming bounds for hyperbolic surfaces" available at
# https://arxiv.org/abs/2302.02540
lambda_max = QQ(0.969)
R_max = QQ(RBF(sqrt(lambda_max-1/4)).upper())

# The half width of the characteristic function of which we take the 4-fold
# convolution
d = L/4

if lambda_max > (pi/d)^2+1/4:
    print("L is too large, so that f^ is not decreasing on the required
    interval.\n")

def fhat(y):
    if y < 1/4:
        R = i*sqrt(1/4-y)
    else:
        R = sqrt(y-1/4)

    H = (sin(d*R)/(d*R))^4
    return H

LHS = RBF(fhat(lambda_max))

print("The value of f^(sqrt(lambda - 1/4)) at the right endpoint of the
interval is bounded below by", LHS.lower(), "\n")

ident = G(1).gap()

# A list of all the irreps that can appear in the first eigenspace and their
# real dimensions
potential_reps = []
potential_dims = []

for m in range(len(characters)):

```



```

phi = G.gap().Irr()[m]

□
↪print("-----")
    print("Representation number", m+1)
□
↪print("-----")
    Cdim = QQ(ident^phi)
    if is_real[m] == True:
        Rdim = Cdim
    else:
        Rdim = 2*Cdim
    print("Complex dimension:", Cdim)
    print("Real dimension:", Rdim)

    # Compute an upper bound for the geometric side of the trace formula:
    RHS = RBF(integral_contribution(d,m))
    RHS += RBF(elliptic_contribution(d,m))
    RHS += RBF(hyperbolic_contribution(d,m,prim_hyp_elts,L))

    # Subtract  $f(i/2)$  for the trivial representation
    if m == 0 :
        RHS -= RBF((sinh(d/2)/(d/2))^4)

    print("The right-hand side in Proposition 3.1 is bounded above by",RHS.
↪upper(),"\n")

    if not LHS > RHS:
        # We cannot verify that  $LHS > RHS$  in Proposition 3.1, so this irrep
↪could appear in the first eigenspace
        potential_reps.append(m)
        potential_dims.append(Rdim)

print("-----")
print("-----")
print("\n\n")
print("The multiplicity of the first eigenvalue is at_
↪least",min(potential_dims))
print("\nThe irreducible representations that could appear are those in the_
↪list",[m+1 for m in potential_reps])

```

The value of  $f(\sqrt{\lambda - 1/4})$  at the right endpoint of the interval is bounded below by 0.760821774497671

-----  
-----

Representation number 1

Complex dimension: 1

Real dimension: 1

The right-hand side in Proposition 3.1 is bounded above by 0.00144333193781869

Representation number 2

Complex dimension: 3

Real dimension: 6

The right-hand side in Proposition 3.1 is bounded above by 0.00585140395102181

Representation number 3

Complex dimension: 3

Real dimension: 6

The right-hand side in Proposition 3.1 is bounded above by 0.00585140395102181

Representation number 4

Complex dimension: 6

Real dimension: 6

The right-hand side in Proposition 3.1 is bounded above by 0.00897221907363559

Representation number 5

Complex dimension: 7

Real dimension: 7

The right-hand side in Proposition 3.1 is bounded above by 0.0659862923862860

Representation number 6

Complex dimension: 7  
Real dimension: 7  
The right-hand side in Proposition 3.1 is bounded above by 0.0442600367731427

-----  
-----  
Representation number 7  
-----  
-----

Complex dimension: 7  
Real dimension: 7  
The right-hand side in Proposition 3.1 is bounded above by 0.429953047100938

-----  
-----  
Representation number 8  
-----  
-----

Complex dimension: 8  
Real dimension: 8  
The right-hand side in Proposition 3.1 is bounded above by 0.392487105832214

-----  
-----  
Representation number 9  
-----  
-----

Complex dimension: 14  
Real dimension: 14  
The right-hand side in Proposition 3.1 is bounded above by 0.0602777784118050

-----  
-----  
Representation number 10  
-----  
-----

Complex dimension: 21  
Real dimension: 21  
The right-hand side in Proposition 3.1 is bounded above by 0.951017064359683

-----  
-----  
Representation number 11  
-----  
-----

Complex dimension: 21  
Real dimension: 21  
The right-hand side in Proposition 3.1 is bounded above by 0.441539593948812

-----  
-----  
-----  
-----

The multiplicity of the first eigenvalue is at least 21

The irreducible representations that could appear are those in the list [10]

[ ]:
